# Supplementary material for: A self-supervised framework for learning whole slide representations
Source: arXiv:2402.06188 source file (2024-05-23)
Supplement: Supplementary file 1 [file supp.results.ssspt.fewshot.tex]

\newcommand\threedsetheaders{& \multicolumn{3}{c}{TCGA BRCA}
                      & \multicolumn{3}{c}{TCGA NSCLC}
                      & \multicolumn{3}{c}{TCGA RCC}}

\begin{table*}[h!]
\setlength{\tabcolsep}{3pt}
\centering{\resizebox{\textwidth}{!}{

\begin{tabular}{cccccccccccccccc}\toprule
\threedsetheaders\\
\cmidrule(lr){2-4}\cmidrule(lr){5-7}\cmidrule(lr){8-10}
&\metricheaders & \metricheaders & \metricheaders\\\midrule
ABMIL        &     61.0 (7.8)  &     34.0 (14.3) &     70.2 (6.1)  &     74.6 (5.0)  &     74.4 (6.4)  &     82.0 (4.3)  &     86.2 (4.7)  &     85.4 (3.6)  &     96.7 (1.2)\\
CLAM         &     72.7 (5.9)  &     52.7 (8.0)  &     79.6 (6.0)  &     76.3 (4.0)  &     76.0 (5.7)  &     85.2 (3.2)  &     83.0 (3.0)  &     81.6 (2.7)  &     95.7 (1.2)\\
DSMIL        &     66.5 (8.9)  &     45.2 (13.9) &     76.0 (8.4)  &     70.0 (5.0)  &     67.0 (8.2)  &     78.7 (6.9)  &     79.9 (8.8)  &     78.3 (6.5)  &     94.9 (2.6)\\
TransMIL     &     72.2 (5.8)  &     53.4 (8.0)  &     83.9 (5.5)  &     85.3 (2.8)  & \tb{85.7 (2.7)} & \tb{92.9 (1.3)} &     86.7 (5.7)  &     85.6 (3.6)  &     96.9 (1.1)\\
HIPT         &     69.0 (8.8)  &     48.7 (16.8) &     82.1 (6.6)  & \tb{86.0 (3.1)} &     85.6 (3.7)  &     92.3 (1.9)  &     89.0 (5.1)  & \tb{88.5 (4.2)} & \tb{97.4 (1.1)}\\
GigaSSL      &     77.2 (5.4)  &     55.7 (5.4)  & \tb{86.7 (6.8)} &     81.7 (5.6)  &     82.6 (5.1)  &     89.9 (3.3)  &     87.5 (2.9)  &     85.2 (2.5)  &     96.5 (0.7)\\
ssSPT (Ours) & \tb{77.9 (4.8)} & \tb{59.6 (3.8)} &     83.7 (5.3)  &     85.2 (3.5)  &     85.3 (3.6)  & \tb{92.9 (2.4)} & \tb{89.4 (4.5)} &     87.3 (4.4)  &     97.1 (1.3)\\\bottomrule
\end{tabular}}}
\caption{\textbf{TODO.} TODO.} 
\label{tab:supp.results.ssspt.fewshot}
\end{table*}
